# Supplementary material for: Multi-Armed Bandit Problem with Temporally-Partitioned Rewards: When Partial Feedback Counts
Source: arXiv:2206.00586 source file (2022-06-01)
Supplement: Supplementary file 1 [file Appendix3_algo.tex]

\section{The \texttt{MR-PD-UCB} Algorithm}
%We propose an algorithm suited for the partially delayed setting when the reward is $\alpha$-smooth and the instantaneous rewards are i.i.d. 

\begin{algorithm}[t!]
	\caption{\texttt{MR-PD-UCB}}
	\begin{algorithmic}[1]						
		\For { $t \in  \{1, \ldots,K\}$} \Comment{init phase}
		\State pull the $t$-th arm in $\mathcal{A}$ 
		\EndFor
		\For { $t \in  \{K+1, \ldots,n\}$} \Comment{loop phase}
		\For { $i \in  \{1, \ldots,K\}$}
		\For { $k \in  \{1, \ldots,\alpha\}$}
		\State $\mathbb{E}[Z^{i}_{k}] \gets \frac{1}{n^i_{k}}\sum_{t:i_t=i}Z^{i}_{t,k}$
		\State $c_{t,n^i_k} \gets \frac{\overline{R}^i}{\alpha}\sqrt{\frac{2\ln t}{n^i_k}}$ 
		\EndFor
		\State $u^i_t \gets \sum_{k=1}^{\alpha}\mleft(\mathbb{E}[Z^{i}_k] + c_{t,n^i_k}\mright) $
		\EndFor
		\State pull arm $i$ such that  $i = \argmax_i$ $u^i_t$
		\EndFor	
	\end{algorithmic}
	\label{a:mr-pd-ucb1}
\end{algorithm}

We present the Multiple-Reward Partially-Delayed UCB algorithm (\emph{i.e.}, \texttt{MR-PD-UCB}) developed for managing the specific case of $\alpha$-smooth and i.i.d. aggregated rewards.
We remark that the $\alpha$-smoothness property only requires the independence between the aggregated rewards.
As a consequence, observing the first samples after the pull is useless to predict the trend on the last ones.
However, in this specific scenario, aggregated rewards are much more informative because they are drawn from the same distribution, therefore, they are exchangeable.
%

%In the presence of partial delay, the idea is that we can simply compute the UCB1 upper confidence bound by only using the observed rewards. Then, at each time instant, we pull the arm with the highest upper confidence bound. Notice that this idea is at the basis of the Delayed-UCB1 algorithm by \cite{joulani2013online}, and we already applied it to the delayed setting in Section \ref{s:delayed}. However, in the partially delayed setting we have to be careful when we take into account the partial observations. Different assumptions on the reward structure allow us to use them in diffent ways.

%In this section, we assume that the instantaneous rewards are i.i.d, therefore agregated rewards give us more information than in the previous setting. In fact, when an arm is pulled, the first instantaneous rewards are sampled from the same distribution of the last ones. As a consequence, instantaneous rewards from the same arm are exchangeable and can be aggregated.

Now, we analyze the worst-case scenario, that is the case in which the number of missing rewards for a given arm is maximized. This happens when we pull the same arm consecutively for $\Tmax$ rounds. In the worst case, the maximum number of missing rewards is $\max\{0,(n_i-\Tmax)\alpha\}$ for the delayed setting, while it is $\lfloor\frac{\alpha(\Tmax-1)}{2}\rfloor$ for the partially delayed setting. From this observations we derive the following theorem.

\begin{theorem}\label{teo:PDAlphaiid}
	For any $t \ge 1$ the expected regret of the Delayed-UCB1 algorithm applied to the setting with Partially Delayed, $\alpha$-smooth reward and i.i.d. instantaneous rewards is bounded by
	%\[\mathbb{E}[\mathfrak{R}_t] \le \sum_{i:\mu_i<\mu^*} \Bigg(\frac{8\Tmax^2\ln{t}}{\alpha^2\Delta_i}\Bigg) + \alpha\Bigg( \frac{\pi^2}{3} + \frac{(\Tmax-1)}{2}\Bigg)\sum_{j=1}^{K} \Delta_j.\] 
	\[\mathbb{E}[\R_t] \le \sum_{i:\mu_i<\mu^*} 
	\mleft( \frac{8(\overline{R}^i)^2\ln(t)}{\alpha\Delta_i} \mright) + \mleft( \frac{\pi^2}{3} + \frac{(\Tmax-1)}{2}\mright)\sum_{j=1}^K \Delta_j.\]
\end{theorem}

\clearpage
